# Supplementary material for: PAPER: Privacy-Preserving Convolutional Neural Networks using Low-Degree Polynomial Approximations and Structural Optimizations on Leveled FHE
Source: arXiv:2509.22857 source file (2026-09-09)
Supplement: Supplementary file 1 [file visual_results.tex]

\section{Visualization of Experimental Results}
\label{sec:visual_results}

Figure \ref{fig:fullpage_results} provides a visual illustration of the experimental results, summarizing the trade-off between accuracy and private inference time across multiple CNN models and datasets, and comparing clustering strategies, ensemble configurations, and baseline methods.


\begin{figure*}
    \centering
    \includegraphics[width=0.845\linewidth]{figures/fullpage_results.eps}
    \caption{\small Accuracy vs. private inference time for VGG and ResNet models on CIFAR and Tiny-ImageNet datasets. Ensembles are evaluated with $M \in \{1, 2, 4\}$ ($M = 1$ is a single model). We compare Standard ensembles (no clustering), Slice ensembles (Slice Clustering), and Full Clustering. Colored squares represent centroid counts ($k = 16, \dots, 8192$), and the same color is used for the same centroid count in both slice and full clustering. Baselines include AutoFHE (numbers = bootstrapping layers) and MPCNN. The green line shows plaintext ReLU accuracy.}
    \label{fig:fullpage_results}
\end{figure*}
